# Supplementary material for: Interplay of Defects and the Charge Density Wave State in Hf-Doped ZrTe$_{3}$
Source: arXiv:2512.17867 ancillary file (2025-12-19)
Supplement: Supplementary file 1 [file ZrTe3_Supplemental_Material.pdf]

## SUPPLEMENTAL MATERIAL

Ghilles Ainouche, Resmi Sudheer, Susree Mohapatra, Boning Yu, Muhammad Suhayb Malik, Yu Liu, Cedomir Petrovic, Abhilash Ravikumar, Michael C. Boyer

## SM1: BIAS DEPENDENT MEASUREMENTS OF DEFECTS

As illustrated in Figure S1, at negative sample biases, from -50 mV to -400 mV, there are two main types of defects evident, and which are detailed in the main manuscript: extended bright defects (EBDs) and extended dark defects (EDDs). Both defects retain their bright/dark character over the negative bias range of the study. However, at positive biases, whereas the EDDs continue to appear dark, the EBDs first appear less bright at +50 mV and +100 mV, then turn dark by +200 mV. This change with bias emphasizes that the extended nature of the EBDs has an important electronic component; were the bright nature purely due to an elevated topographic nature, one would expect the EBD to remain bright at positive biases.

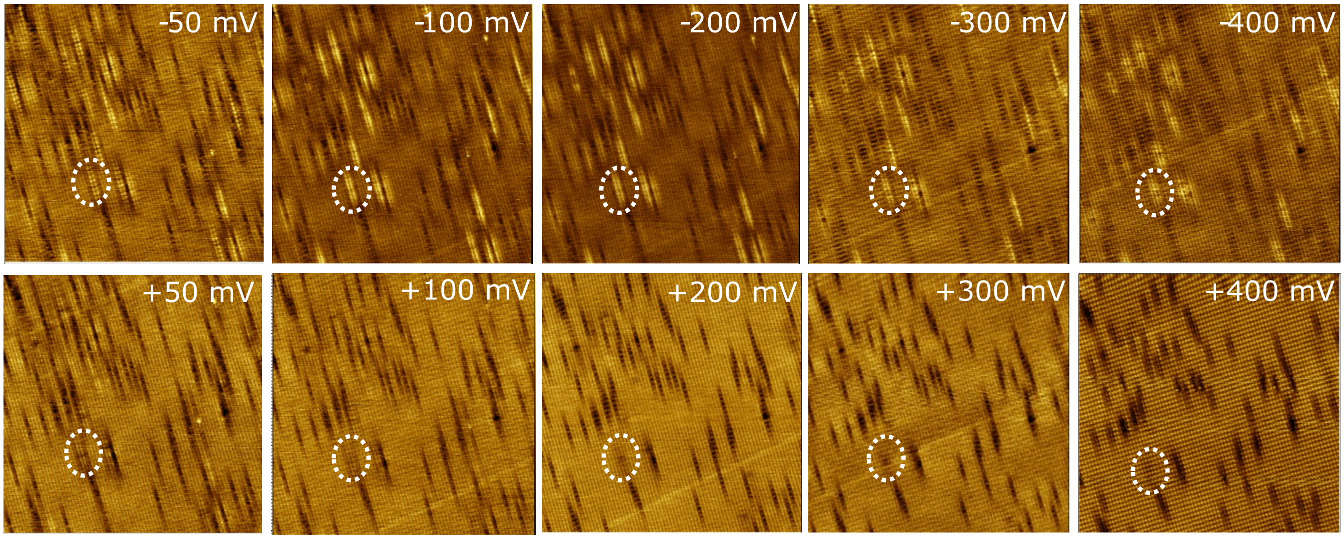


FIG. S1. Topographic images acquired over the same 38 nm x 38 nm region. I = 50 pA. A single defect is circled in white. This defect, while appearing as an EBD at negative biases becomes dark at positive biases (+200 mV and above).

## SM2: Te SUBSURFACE VACANCY

Using DFT, we simulate the topographic appearance of a subsurface Te vacancy and present this simulation side-by-side with a suspected Te subsurface vacancy detected in STM our topographic measurements (Figure S2). In the STM-acquired topography (Figure S2a), a possible defect is identified by a slight disruption in the positioning of four surface Te ions leading to a slightly enlarged 'dark' region at the center of those ions as compared to the center of other surface Te ions.

In (Figure S2b), the relaxed crystal structure is overlaid on the STM topography with four Te ions highlighted in orange to emphasize the position of the subsurface Te vacancy. The resulting simulated STM image (Figure S2c) shows the effect the subsurface Te vacancy is relatively localized. It does not have the extended nature as seen for the EBD or EDD defects leading us to conclude that the EBDs and EDDs are not due to subsurface Te vacancies. Rather, the defect leads to a slightly extended dark region at the center of the four neighboring Te ions. Linecuts through the acquired and simulated STM images show general agreement providing support for the identification of a subsurface Te defect in STM measurements.

We note that due to the much more local and subtle effect that a Te vacancy has on the topography, it is more difficult to identify these defects in STM topographies, provide statistics, or determine whether the CDW state is obviously correlated with these defects.

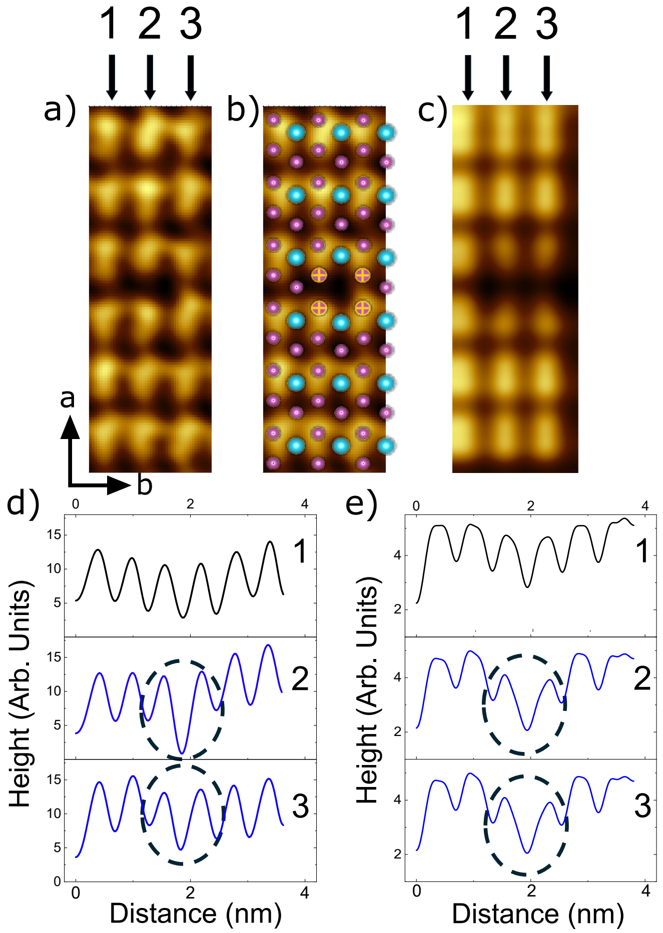


FIG. S2. Subsurface Te Vacancy a) Zoom-in on a suspected subsurface Te vacancy identified in an STM-acquired topography (I = 50 pA, $V_{Sample}$ = -50 mV). 5 pixel Gaussian smoothing of the topography is used to visibly aid in identifying the location of the suspected defect. b) Overlay of the relaxed crystal structure on the STM image from a). c) DFT-simulated STM image at -50 mV. The dimmer ions at the center, representing the nearest neighbors, are highlighted in b). To aid in comparison to the topography in a), we applied similar Gaussian smoothing to the simulated image. d) Line cuts taken vertically (along the $a$-axis) through the three atomic columns in the STM topography of a). The black line cut is away from the defect region (left atomic column). The two blue line cuts are taken through the middle and right atomic columns illustrating Te ion variations near a suspected Te vacancy. e) Identical line cuts through the simulated topography of c). The circled peaks in d) and e) correspond to suspected or simulated defect region.

## SM3: DEFECT IDENTIFICATION

We identify the location of defects using two techniques which evince similar results: 1) FFT signal extraction and 2) template matching.

*FFT signal extraction*: Because defects are not periodically arranged in a topography, the signal associated with the defects is not as easily discerned as with atomic or CDW periodicities. For $ZrTe_3$, the signal associated with defects in the FFT of a topographic image is mainly within a diffuse cloud extending mainly along the $b$*-axis, though additional contributions outside of this region are possible.

Figure S3 shows a topography of $ZrTe_3$ with EBDs and EDDs. We Fourier filter the image to include the signal within the rectangle of Figure S3b but excluding the CDW signals within the ovals. What results is an image free of atomic and CDW signals helping to enhance defect signals. Next, we can then identify the EBDs and EDDs using intensity thresholding so as to extract their individual locations (Figure S3c and d) and determine the center of defects (Figure S3e and f).

*Template Matching*: In template matching (Figure S4), we use an EBD and an EDD image cropped from a topography as a template to which other defect candidates in the topography are compared. To aid in identification

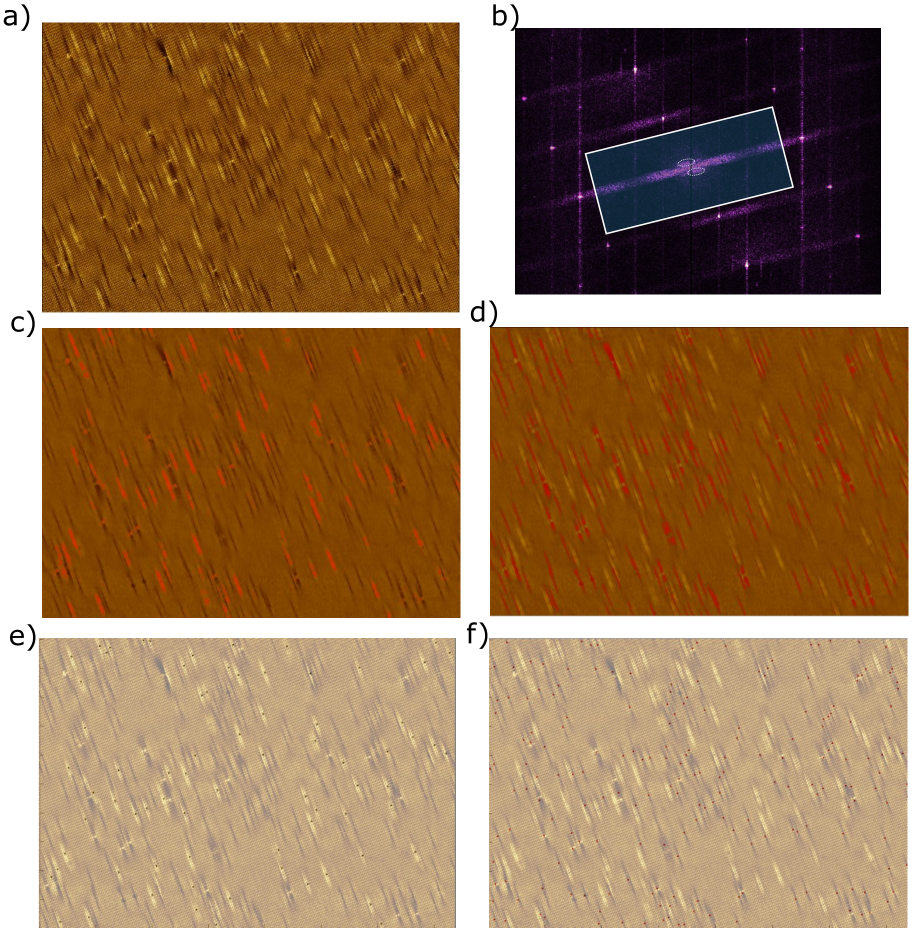


FIG. S3. Identifying defects using Fourier filtering (a) High-resolution 60 nm x 92 nm topography (I = 50 pA, $V_{Sample}$ = -50 mV). (b) FFT of the image shown in (a). We Fourier filter the topography to include the signal within the white rectangle while excluding the CDW signal within the white ovals which results in figures c) and d). (c)-(d) Fourier filtered topography with EBDs (c) and EDDs (d) identified using intensity thresholding. (e)-(f) Centers of the of EBDs e) and EDDs f) identified using this methodology.

of defects the CDW signal is removed from the topography using Fourier filtering and the atomic signal is reduced using Gaussian smoothing ($\sim$ 0.6 nm). These steps help to enhance the defect signal in the images. The identification of defects within an image are made by carrying out the normalized cross-correlation of the EBD (or EDD) defect and the topographic image. Points in the resulting cross-correlation map with values of $\sim$ 0.6 or above typically indicate a defect match.

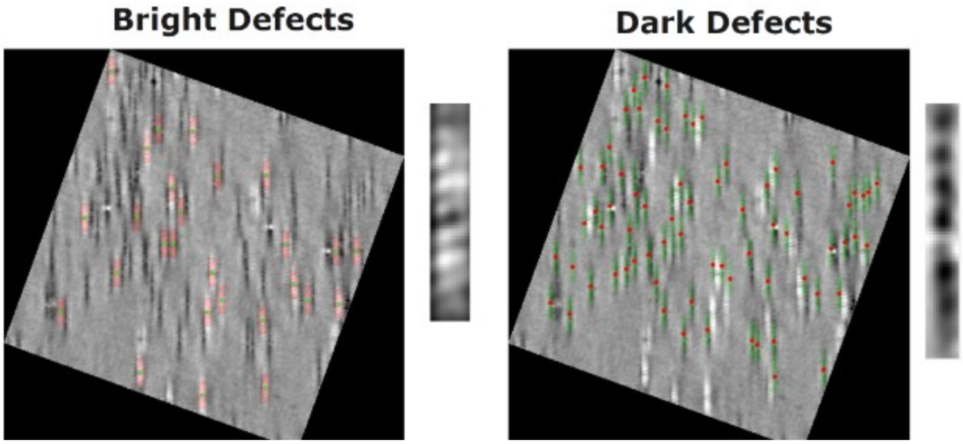


FIG. S4. Identifying defects using Fourier filtering. At left, a topography with corresponding EBD template. Defect matches are identified by red rectangles and the defect center with green. At right, the same topography with a corresponding EDD template. Defect matches are identified by green rectangles and the defect center with a red circle. We find it helpful to have the $a$-crystal axis vertical when carrying out template matching given the extended nature of the defects along the $a$-axis.
